# Supplementary material for: Taming Recommendation Bias with Causal Intervention on Evolving Personal Popularity
Source: arXiv:2505.14310 source file (2025-05-28)
Supplement: Supplementary file 1 [file appendix.tex]

\section{Baselines}
\label{app:baselines}

\begin{itemize}[leftmargin=15pt]
\item \underline{\textbf{IPS}}~\cite{DBLP:conf/ijcai/JoachimsSS18,DBLP:conf/icml/SchnabelSSCJ16}: eliminates popularity bias by re-weighting each instance based on item popularity. To reduce variance, a max-capping trick is applied to the IPS values~\cite{DBLP:journals/jmlr/BottouPCCCPRSS13}.
\item \underline{\textbf{UDIPS}}~\cite{DBLP:conf/sigir/LuoW23} considers the user's sensitivity toward popularity, but %differently 
it is time-irrelevant and is not for popular items only. UPIPS conducts propensity scores rather than deconfounded training to achieve debiasing. 
\item \underline{\textbf{MACR}}~\cite{DBLP:conf/kdd/WeiFCWYH21} performs counterfactual inference to remove the direct effect of item popularity from the item node to the ranking score.
\item  \underline{\textbf{PPAC}}~\cite{DBLP:conf/www/NingC0KHH024} splits popularity bias into global and personal popularity. This distinction allows for redefining popular items for each user, acknowledging that some items may be popular only within specific user groups rather than be overall popular.
\item \underline{\textbf{DICE}}~\cite{DBLP:conf/www/ZhengGLHLJ21} disentangles user preference and popularity bias into two sets of embeddings.
\item \underline{\textbf{PD}}~\cite{DBLP:conf/sigir/ZhangF0WSL021} performs deconfounded training by intervening in popularity bias during model inference. PD uses the matching score directly for recommendations.
\item \underline{\textbf{PDA}}~\cite{DBLP:conf/sigir/ZhangF0WSL021} performs deconfounded training by intervening in popularity bias during model inference. PDA incorporates a predicted item popularity score into the recommendation process.
\item \underline{\textbf{TIDE}}~\cite{DBLP:journals/tkde/ZhaoCZHCZW23} disentangles popularity bias into two parts for recommendation: the benign part, which represents the time-invariant quality of items, and the harmful part, which reflects the time-aware conformity of items.
\item \underline{\textbf{PARE}}~\cite{DBLP:conf/cikm/JingZ0023} accounts for temporal fluctuations in item popularity during training through three key modules: Popularity History Module, which captures the evolution in popularity; Temporal Impact Module, which encodes relevant time information; and Periodic Impact Module, which encodes the current time information. %To ensure a fair comparison, we exclude embeddings for category and other side information, retaining only the ID and time information, consistent with other baselines. 
\end{itemize}

\section{Intuition of Local Popularity}
\label{app:local_pop}

The intuition for splitting global and local popularity is that items share similar global popularity (around $600$) while their local popularity trends differ, as shown in Figure~\textcolor{blue}{\ref{fig:short-term_popularity}}. For example, item ``1857'' is popular around 2011, while item ``792'' gains local popularity around 2015. If we recommend items according to local popularity, we prefer to suggest item ``792'' since it is popular recently. 

\begin{figure}[ht]
	\centering
        \includegraphics[scale=0.5]{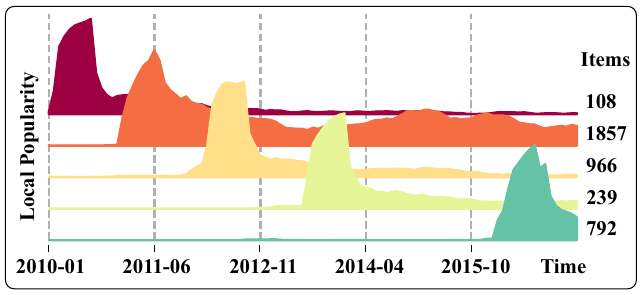}
    \vspace{-8pt}
	\caption{Temporal evolution of local popularity for five items on Douban-Movie. Local popularity refers to the item popularity over the past half-year. }
    \label{fig:short-term_popularity}
    \vspace{-5pt}
\end{figure}

\section{Consistency Ratio}
\label{app:consistency_ratio}
The example of consistency ratio is shown in Figure~\textcolor{blue}{\ref{fig:conformity_weight}}. As $\alpha$ increases, the score becomes more sensitive to the gap between personal popularity $s_u^t$ and local popularity $p_i^t$. 

\begin{figure}[h]
	\centering
        \includegraphics[scale=0.4]{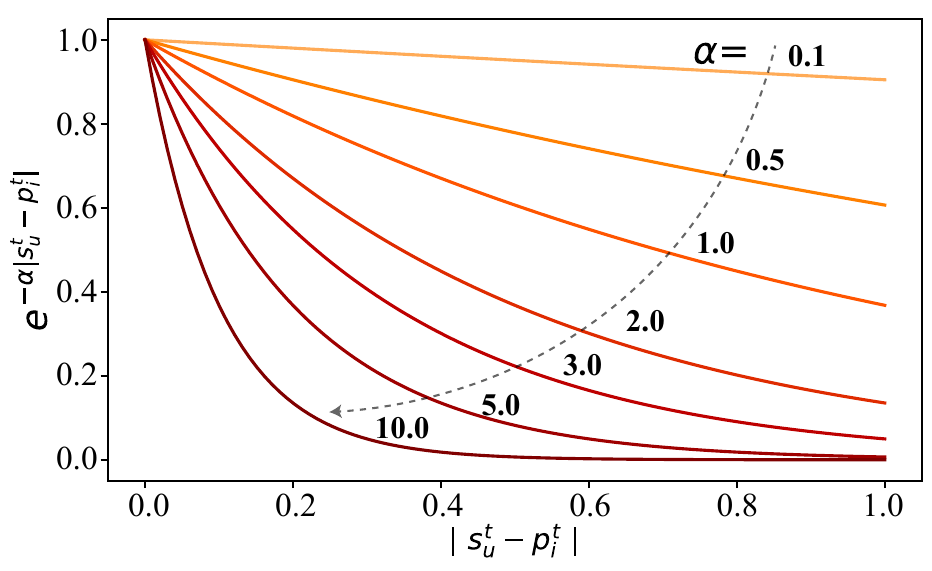}
        \vspace{-8pt}
	\caption{The consistency score varies with different values of $\alpha$. As $\alpha$ increases, the score becomes more sensitive to the gap between personal popularity $s_u^t$ and local popularity $p_i^t$.}
    \label{fig:conformity_weight}
\end{figure}

\section{Example of temporal evolution}
\label{app:evolution}
Example of temporal evolution on both local popularity and popularity sensitivity. 
As shown in Figure~\textcolor{blue}{\ref{fig:ma_popularity_and_sensitivity}}, item 17's local popularity and user 521's personal popularity fluctuated over time (blue line). The orange line represents the moving average, while the trend is indicated by the gradient of the moving average line.
We observe the trend of evolution, and predict the future values of both local popularity and personal popularity. Finally, we intervene the local popularity and personal popularity to recommend item $17$ to user $521$. 

\begin{figure}[h]
	\centering
        \includegraphics[scale=0.28]{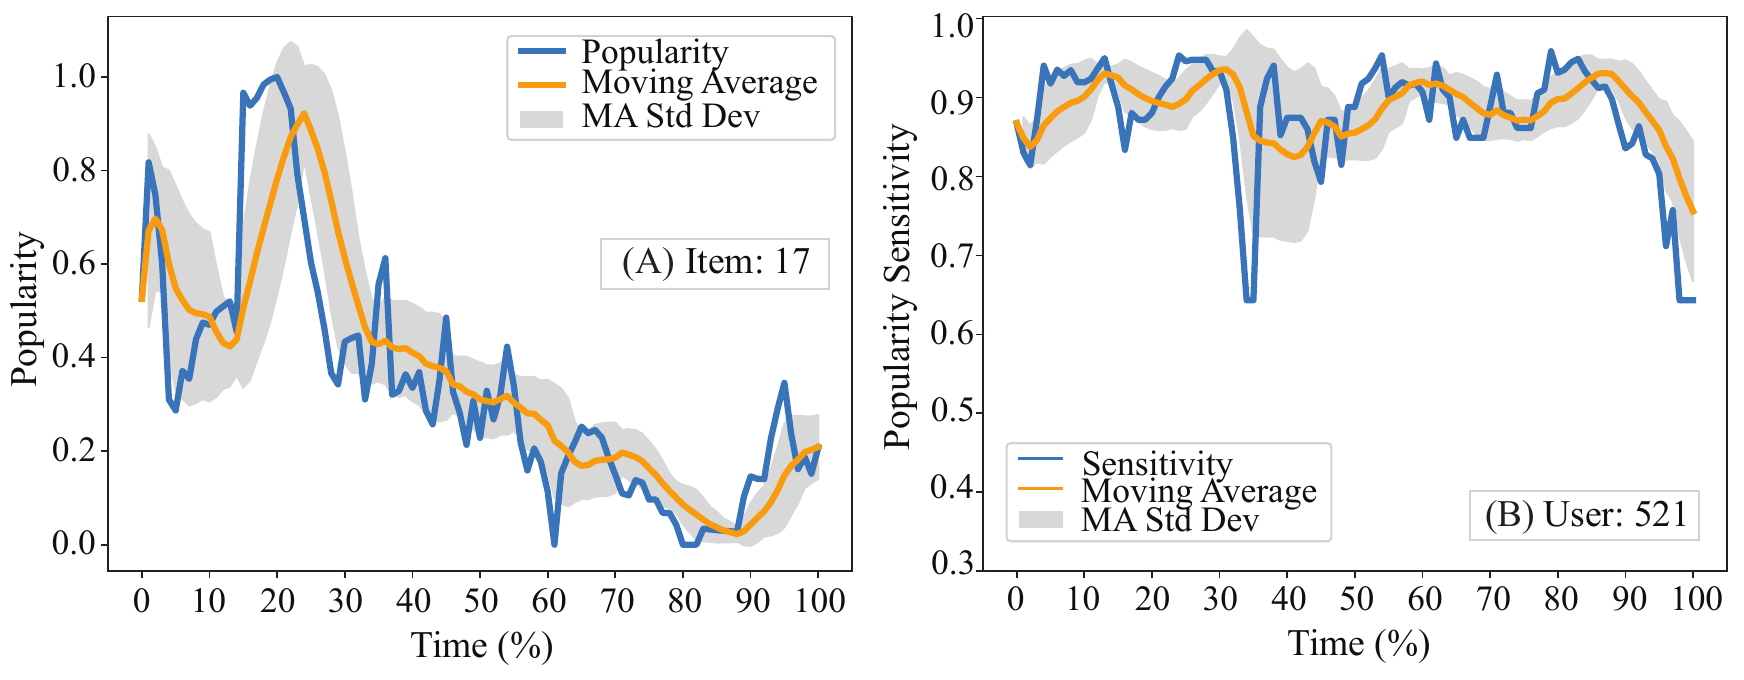}
        \vspace{-8pt}
	\caption{
    Temporal evolution of both local popularity and popularity sensitivity. (A): The local popularity of Item $17$ has an upward trend. (B): The popularity sensitivity of user $521$ has an downward trend.}
    \label{fig:ma_popularity_and_sensitivity}
\end{figure}

\vspace{-8pt}
\section{\tsy{Further experiments}}
We provide additional results with another backbone model (NCF), on the Ciao and MovieLens-1M datasets. For MovieLens dataset, we do not follow the same split setting as PPAC, which applies random splitting, restricts test users with more than 30 interactions, and uses 3-core filtering. Instead, we follow the chronological split described in Section~\ref{subsec:experiment_setting}, where the dataset is divided into 10 parts (first nine parts for training and the last part for validation and testing). The evaluation is Recall@20, Precision@20, NDCG@20.

\begin{table}[ht]
\centering
\caption{Performance Comparison with another backbone model (NCF). The notations are the same as those in Table~\textcolor{blue}{\ref{tab:performance_comparison_lightgcn}}.}
\resizebox{0.47 \textwidth}{!}
{
\begin{tabular}{l|ccc|ccc}
\toprule
%\rowcolor{gray!20}
Datasets    & \multicolumn{3}{c|}{Ciao}       & \multicolumn{3}{c}{ MovieLens-1M} \\ 
Metrics     & Rec@20 & Pre@20 & NDCG@20  & Rec@20 & Pre@20 & NDCG@20  \\ 
 \midrule \midrule
NCF        & 0.0248 & 0.0079 & 0.0095 & 0.0708 & 0.2008 & 0.2102 \\
IPS        & 0.0224 & 0.0092 & 0.0110 & 0.0650 & 0.1976 & 0.2053 \\
PDA        & \underline{\textcolor{violet}{0.0259}} & 0.0109 & \underline{\textcolor{violet}{0.0124}} & \underline{\textcolor{violet}{0.0750}} & \underline{\textcolor{violet}{0.2108}} & 0.2203 \\
TIDE       & 0.0255 & \underline{\textcolor{violet}{0.0112}} & 0.0096 & 0.0714 & 0.2055 & 0.2138 \\
PPAC       & 0.0253 & 0.0109 & 0.0102 & 0.0705 & 0.2067 & \textbf{\textcolor{brightmaroon}{0.2274}} \\
CausalEPP  & \textbf{\textcolor{brightmaroon}{0.0314}} & \textbf{\textcolor{brightmaroon}{0.0122}} & \textbf{\textcolor{brightmaroon}{0.0125}} & \textbf{\textcolor{brightmaroon}{0.0799}} & \textbf{\textcolor{brightmaroon}{0.2140}} & \underline{\textcolor{violet}{0.2265}} \\
\bottomrule
\end{tabular}
}
\end{table}
